# Supplementary material for: One Law, Many Languages: Benchmarking Multilingual Legal Reasoning for Judicial Support
Source: arXiv:2306.09237 source file (2024-08-21)
Supplement: Supplementary file 1 [file datasheet.tex]

\section{Data sheet}
%https://arxiv.org/pdf/1803.09010.pdf
\label{app:datasheet}
\subsection{Motivation}

\textcolor{blue}{\textbf{For what purpose was the dataset created?} Was there a specific task in mind? Was there a specific gap that needed to be filled? Please provide a description.} Comprehensive study of the usage of NLP methods for supporting non-English, inherently multilingual, federal legal system.

\textcolor{blue}{\textbf{Who created the dataset (e.g., which team, research group) and on behalf of which entity (e.g., company, institution, organization)?}} The dataset was created by Joel Niklaus (University of Bern, Bern University of Applied Sciences, Stanford University), Vishvaksenan Rasiah (University of Bern), Ronja Stern (University of Bern), and Veton Matoshi. (Bern University of Applied Sciences) 

\textcolor{blue}{\textbf{Who funded the creation of the dataset?} If there is an associated grant, please provide the name of the grantor and the grant name and number.} This work has been supported by the Swiss National Research Programme “Digital Transformation” (NRP-77) grant number 187477.

\textcolor{blue}{\textbf{Any other comments?}} None.

\subsection{Composition}
\textcolor{blue}{\textbf{What do the instances that comprise the dataset represent (e.g., documents, photos, people, countries)?} Are there multiple types of instances (e.g., movies, users, and ratings; people and interactions between them; nodes and edges)? Please provide a description.} The dataset consists of Swiss court cases scraped from \href{www.Entscheidsuche.ch}{Entscheidsuche.ch}.

\textcolor{blue}{\textbf{How many instances are there in total (of each type, if appropriate)?}} There are 638K court rulings, and 36K laws.

\textcolor{blue}{\textbf{Does the dataset contain all possible instances or is it a sample (not necessarily random) of instances from a larger set?} If the dataset is a sample, then what is the larger set? Is the sample representative ofthe larger set (e.g., geographic coverage)? If so, please describe how this representativeness was validated/verified. If it is not representative of the larger set, please describe why not (e.g., to cover a more diverse range of instances, because instances were withheld or unavailable).} The dataset comprises a sample of Swiss court cases, which were scraped from \href{www.Entscheidsuche.ch}{Entscheidsuche.ch} over a specific time period. Although we did not formally validate the representativeness of the sample, we assert its representativeness based on the fact that we scraped every new court decision published within that time frame.

\textcolor{blue}{\textbf{What data does each instance consist of?} “Raw” data (e.g., unprocessed text or images) or features? In either case, please provide a description.} Each instance in the dataset is a court decision. The composition of each instance varies depending on the task, such as text classification or information retrieval, by including special labels or additional information (e.g., queries). For more details, please refer to Section \ref{sec:datasets}.

\textcolor{blue}{\textbf{Is there a label or target associated with each instance?} If so, please provide a description.} Each instance in the dataset is a court decision. The composition of each instance varies depending on the task, such as text classification or information retrieval, by including special labels or additional information (e.g., queries). For more details, please refer to Section \ref{sec:datasets}.

\textcolor{blue}{\textbf{Is any information missing from individual instances?} If so, please provide a description, explaining why this information is missing (e.g., because it was unavailable). This does not include intentionally removed information, but might include, e.g., redacted text.} No.

\textcolor{blue}{\textbf{Are relationships between individual instances made explicit (e.g., users’ movie ratings, social network links)? } If so, please describe how these relationships are made explicit.} The dataset does not require any relationships between individual instances to be made explicit, unless they are necessary for the specific task at hand.

\textcolor{blue}{\textbf{Are there recommended data splits (e.g., training, development/validation, testing)} If so, please provide a description of these splits, explaining the rationale behind them.} See Section \ref{tab:lextreme-task-dist}.

\textcolor{blue}{\textbf{Are there any errors, sources of noise, or redundancies in the dataset? If so, please provide a description.}} Not that we know of.

\textcolor{blue}{\textbf{Is the dataset self-contained, or does it link to or otherwise rely on external resources (e.g., websites, tweets, other datasets)} If it links to or relies on external resources, a) are there guarantees that they will exist, and remain constant, over time; b) are there official archival versions of the complete dataset (i.e., including the external resources as they existed at the time the dataset was created); c) are there any restrictions (e.g., licenses, fees) associated with any of the external resources that might apply to a dataset consumer? Please provide descriptions of all external resources and any restrictions associated with them, as well as links or other access points, as appropriate.} The dataset is self-contained.

\textcolor{blue}{\textbf{Does the dataset contain data that might be considered confidential (e.g., data that is protected by legal privilege or by doctor–patient confidentiality, data that includes the content of individuals’ non-public communications) If so, please provide a description.}} No. The dataset is derived from court decisions that are published by official authorities, making it very unlikely to contain confidential information.

\textcolor{blue}{\textbf{Does the dataset contain data that, if viewed directly, might be offensive, insulting, threatening, or might otherwise cause anxiety?} If so, please describe why.}  No. The dataset is derived from court decisions that are published by official authorities, making it very unlikely to have content that might be offensive, insulting, threatening, or might otherwise cause anxiety.

\textcolor{blue}{\textbf{Does the dataset identify any subpopulations (e.g., by age, gender)?} If so, please describe how these subpopulations are identified and provide a description of their respective distributions within the dataset.} Not that we know of. The dataset, derived from court decisions published by official authorities, is very unlikely to identify any subpopulation. 

\textcolor{blue}{\textbf{Is it possible to identify individuals (i.e., one or more natural persons), either directly or indirectly (i.e., in combination with other data) from the dataset?}If so, please describe how.} To the best of our knowledge, it is not possible to directly or indirectly identify individuals from the dataset. If at all feasible, doing so would require significant effort and additional data.

\textcolor{blue}{\textbf{Does the dataset contain data that might be considered sensitive in any way (e.g., data that reveals race or ethnic origins, sexual orientations, religious beliefs, political opinions or union memberships, or locations; financial or health data; biometric or genetic data; forms of government identification, such as social security numbers; criminal history)?} If so, please provide a description.} To the best of our knowledge, the dataset does not contain data that might be considered sensitive in any way.

\textcolor{blue}{\textbf{Any other comments?}} None.

\subsection{Collection Process}

\textcolor{blue}{\textbf{How was the data associated with each instance acquired? Was the data directly observable (e.g., raw text, movie ratings), reported by subjects (e.g., survey responses), or indirectly inferred/derived from other data (e.g., part-of-speech tags, model-based guesses for age or language)? If the data was reported by subjects or indirectly inferred/derived from other data, was the data validated/verified? If so, please describe how.}} In general, all data were directly observable. We made use of regular expressions to derive labels.

\textcolor{blue}{\textbf{What mechanisms or procedures were used to collect the data (e.g., hardware apparatuses or sensors, manual human curation, software programs, software APIs)?} How were these mechanisms or procedures validated?} We utilized open-source Python libraries for data scraping from Entscheidsuche.ch. Specifically, we employed BeautifulSoup and tika-python libraries to parse HTML and PDF content, respectively. We used metadata from entscheidsuche and regular expressions for semi-automated extraction of ground truth from the underlying text. The choice of these libraries was based on their widespread use and reliability in data scraping and parsing tasks. We did not perform separate validation of these tools, relying on their established performance and accuracy in similar tasks. We manually inspected samples to validate the data.

\textcolor{blue}{\textbf{If the dataset is a sample from a larger set, what was the sampling strategy (e.g., deterministic, probabilistic with specific sampling probabilities)?}} We scraped court decisions from Entscheidsuche.ch over a specific time period without employing any filtering mechanisms. As a result, the sample is arbitrary. 

\textcolor{blue}{\textbf{Who was involved in the data collection process (e.g., students, crowdworkers, contractors) and how were they compensated (e.g., how much were crowdworkers paid)?}} The contributors listed in the paper did the main work of the data collection process. Additionally, students helped with early parts of the data collection as part of their bachelor theses. University employees, paid standard Swiss salaries, also contributed parts of the data collection.

\textcolor{blue}{\textbf{Over what timeframe was the data collected?}} We started the original data collection on December 15, 2020 (first code commit). The data collection process finished on August 31, 2023 (last HuggingFace dataset update commit).

\textcolor{blue}{\textbf{Were any ethical review processes conducted (e.g., by an institutional review board)?}} No.

\textcolor{blue}{\textbf{Any other comments?}} None.

\subsection{Preprocessing/cleaning/labeling}

\textcolor{blue}{\textbf{Was any preprocessing/cleaning/labeling of the data done (e.g., discretization or bucketing, tokenization, part-of-speech tagging, SIFT feature extraction, removal of instances, processing of missing values)? If so, please provide a description.} If not, you may skip the remaining questions in this section.} We scrape all files from \href{www.Entscheidsuche.ch}{Entscheidsuche.ch}, including each court's folder metadata. Only new case documents are sent through the pipeline. \textbf{(2)} We used BeautifulSoup / tika-python library to extract text from HTML / PDF. \textbf{(3)} Language is identified using fastText \citep{grave2018learning} for subsequent tasks. \textbf{(4)} A cleaner removes irregular patterns or redundant text to avoid extraction errors. \textbf{(5)} Cases are segmented into header, facts, considerations, rulings, and footer via regex patterns. \textbf{(6)} To extract the judgement outcome, a word set is defined for each outcome. As these indicators are not context-exclusive, considering only the ruling section is crucial to avoid false positives. Therefore, accurate judgment outcome extraction relies on precise section splitting. \textbf{(7)} \ac{LD} and law citations are obtained through Regex (cantonal) or BeautifulSoup (federal). The \ac{SFCS} labels citations with HTML tags, ensuring a high quality of citations for federal cases. 

\textcolor{blue}{\textbf{Was the “raw” data saved in addition to the preprocessed/cleaned/labeled data (e.g., to support unanticipated future uses)?}} No. The raw data can always be downloaded again from entscheidsuche.ch and fedlex.admin.ch.

\textcolor{blue}{\textbf{Is the software that was used to preprocess/clean/label the  data available?}} Yes. It can be accessed here: URL released upon acceptance. %\href{https://github.com/JoelNiklaus/SwissCourtRulingCorpus}{https://github.com/JoelNiklaus/SwissCourtRulingCorpus}.

\textcolor{blue}{\textbf{Any other comments?}} None.

\subsection{Uses}

\textcolor{blue}{\textbf{Has the dataset been used for any tasks already?} Ifso, please provide a description.} Yes, please refer to Section \ref{sec:datasets}.

\textcolor{blue}{\textbf{Is there a repository that links to any or all papers or systems that use the dataset?} If so, please provide a link or other access point.} No.

\textcolor{blue}{\textbf{What (other) tasks could the dataset be used for?}} As far as we can determine, there are no other tasks for which the dataset can be used without further changes or additions.

\textcolor{blue}{\textbf{Is there anything about the composition of the dataset or the way it was collected and preprocessed/cleaned/labeled that might impact future uses?} For example, is there anything that a dataset consumer might need to know to avoid uses that could result in unfair treatment of individuals or groups (e.g., stereotyping, quality of service issues) or other
risks or harms (e.g., legal risks, financial harms)? If so, please provide a description. Is there anything a dataset consumer could do to mitigate these risks or harms?} Users must be aware that the dataset consists of court decisions from Switzerland. Therefore, any model or application developed based on this dataset should be considered applicable primarily within the context of Swiss law. Applying it to texts from other jurisdictions might yield less favorable results.

\textcolor{blue}{\textbf{Are there tasks for which the dataset should not be used?} If so, please provide a description.} The dataset is specifically tailored for tasks within the context of Swiss law. Therefore, it should not be used for tasks that fall outside this legal framework.

\textcolor{blue}{\textbf{Any other comments?}} None.

\subsection{Distribution}

\textcolor{blue}{\textbf{Will the dataset be distributed to third parties outside of the entity (e.g., company, institution, organization) on behalf of which the dataset was created?} If so, please provide a description.} The dataset is publicly available on HuggingFace (URL released upon acceptance). %\href{https://huggingface.co/collections/joelniklaus/scale-datasets-6535da6123e0af0e0da0b142}{HuggingFace}.

\textcolor{blue}{\textbf{How will the dataset will be distributed (e.g., tarball on website, API, GitHub)?} Does the dataset have a digital object identifier (DOI)?} The dataset is publicly available on HuggingFace (URL released upon acceptance) %\href{https://huggingface.co/collections/joelniklaus/scale-datasets-6535da6123e0af0e0da0b142}{HuggingFace}
, and as such, it can be accessed via an API.

\textcolor{blue}{\textbf{When will the dataset be distributed?}} It is already publicly available.

\textcolor{blue}{\textbf{Will the dataset be distributed under a copyright or other intellectual property (IP) license, and/or under applicable terms of use (ToU)?} If so, please describe this license and/or ToU, and provide a link or other access point to, or otherwise reproduce, any relevant licensing terms or ToU, as well as any fees associated with these restrictions.} The dataset is published under the cc-by-sa-4.0 license.

\textcolor{blue}{\textbf{Have any third parties imposed IP-based or other restrictions on the data associated with the instances?} If so, please describe these restrictions, and provide a link or other access point to, or otherwise reproduce, any relevant licensing terms, as well as any fees associated with these restrictions.} No.

\textcolor{blue}{\textbf{Do any export controls or other regulatory restrictions apply to the dataset or to individual instances?} If so, please describe these restrictions, and provide a link or other access point to, or otherwise reproduce, any supporting documentation.} No.

\textcolor{blue}{\textbf{Any other comments?}} None.

\subsection{Maintenance}

\textcolor{blue}{\textbf{Who will be supporting/hosting/maintaining the dataset?}} The dataset is publicly available on HuggingFace (URL released upon acceptance) %\href{https://huggingface.co/collections/joelniklaus/scale-datasets-6535da6123e0af0e0da0b142}{HuggingFace} 
which will host and maintain the dataset. The code for creating and updating the dataset is open source and available on GitHub (URL released upon acceptance). %\href{https://github.com/JoelNiklaus/SwissCourtRulingCorpus/}{GitHub}.

\textcolor{blue}{\textbf{How can the owner/curator/manager of the dataset be contacted (e.g., email address)?}} The creators of the dataset can be reached through the email address provided in the associated publication or via their Huggingface profile.

\textcolor{blue}{\textbf{Is there an erratum?} If so, please provide a link or other access point.} No.

\textcolor{blue}{\textbf{Will the dataset be updated (e.g., to correct labeling errors, add new instances, delete instances)?} If so, please describe how often, by whom, and how updates will be communicated to dataset consumers (e.g., mailing list, GitHub)?} Currently, there are no plans for updating the dataset, since it is a benchmark. If we update it with new data, we would need to rerun all models, and old numbers would be invalid.

\textcolor{blue}{\textbf{If the dataset relates to people, are there applicable limits on the retention of the data associated with the instances (e.g., were the individuals in question told that their data would be retained for a fixed period of time and then deleted)?} If so, please describe these limits and explain how they will be enforced.} The dataset does not relate to people.

\textcolor{blue}{\textbf{Will older versions ofthe dataset continue to be supported/hosted/maintained?} If so, please describe how. If not, please describe how its obsolescence will be communicated to dataset consumers.} Currently, there are no plans for updating the dataset.

\textcolor{blue}{\textbf{If others want to extend/augment/build on/contribute to the dataset, is there a mechanism for them to do so?} If so, please provide a description. Will these contributions be validated/verified? If so, please describe how. If not, why not? Is there a process for communicating/distributing these contributions to dataset consumers? If so, please provide a description.} Contributors may open pull requests on our GitHub and HuggingFace repos for updating the code or data respectively. Since the funding of the project is over in May 2024, we cannot guarantee the validation/verification afterwards.

\textcolor{blue}{\textbf{Any other comments?}} None.
