# Supplementary material for: One Law, Many Languages: Benchmarking Multilingual Legal Reasoning for Judicial Support
Source: arXiv:2306.09237 source file (2024-08-21)
Supplement: Supplementary file 2 [file data_card.tex]

\section{Data Card}
%https://sites.research.google/datacardsplaybook/
\label{app:datacard}

Given that the dataset comprises a collection of distinct tasks, i.e., datasets, each with different objectives, labels, and statistics, we have not compiled a single data card. Instead, we refer readers to the individual dataset descriptions for each task, which are available on HuggingFace (URL released upon acceptance). %\href{https://huggingface.co/collections/joelniklaus/scale-datasets-6535da6123e0af0e0da0b142}{Hugging Face}. 
